# Supplementary material for: GND: Global Navigation Dataset with Multi-Modal Perception and Multi-Category Traversability in Outdoor Campus Environments
Source: arXiv:2409.14262 source file (2025-03-05)
Supplement: Supplementary file 1 [file appendix.tex]

\section{Supplement}
\label{sec:supplement}
